# Supplementary material for: UniMix: Towards Domain Adaptive and Generalizable LiDAR Semantic Segmentation in Adverse Weather
Source: arXiv:2404.05145 source file (2024-04-08)
Supplement: Supplementary file 1 [file X_suppl.tex]

%\clearpage
%\setcounter{page}{1}
%\maketitlesupplementary

In this Appendix, we supplement more content from the following aspects to support the findings in the main body of this paper:
\begin{itemize}
    \item Sec.~\ref{secA} provides more implementation details of UniMix.
    \item Sec.~\ref{secB} elaborates the empirical studies on the hyper-parameters in universal mixing.
    \item Sec.~\ref{secC} discusses the difference between our universal mixing and other point cloud mixing methods.
    \item Sec.~\ref{secD} provide more technical details of Bridge Domain construction and the visualizations.
    \item Sec.~\ref{secE} analyzes the various mixing methods and visualizes the mixing masks.
    \item Sec.~\ref{secF} shows the comparison of qualitative results.
    % \item Sec. \ref{secG} visualizes the feature represenations.
    \item Sec.~\ref{secH} discusses the limitations and social impact.
\end{itemize}

\section{Implementation Details}\label{secA}
We implemented UniMix in PyTorch and ran our experiments on 2$\times$NVIDIA A100 GPU. We use MinkowskiNet \cite{choy20194d} as our point cloud segmentation network. Specifically, we adopt MinkUNet32 following prior works \cite{saltori2022cosmix_eccv,saltori2022cosmix,xiao2022transfer} for both the teacher and student networks. Before adaptation and generalization, we warm up the network on the source domain with Dice loss \cite{jadon2020survey} for 10 epochs, training from scratch. In UDA and DG, we initialize student and teacher networks with the parameters obtained after warm-up. The warm-up and adaptation stages share the same hyper-parameters. In both the pre-training and adaptation stages, we use Stochastic Gradient Descent (SGD) with a learning rate of 0.001. We use a batch size of 4 for both training stages and train for 10 epochs and 50 epochs for the first and second stages, respectively. We adopt the same data augmentation strategies as typical LiDAR segmentation literature \cite{choy20194d,saltori2022cosmix,saltori2022cosmix_eccv}, including local augmentation and global augmentations. Regarding the parameters selection and setting in the
bridge domain generation process, the critical parameter for simulating light fog and dense fog is the ``attenuation coefficient," representing fog density. Values are randomly selected from the predefined set in \cite{hahner2021fog} (0.005, 0.01, 0.02, 0.03, 0.06) and (0.1, 0.12, 0.15, 0.2), respectively, to enhance data diversity. For rain effect generation, we adapt snow simulation functions from \cite{hahner2022lidar} with reference to the LISA framework \cite{kilic2021lidar}. Key parameters for snow and rain simulations, namely ``snowfall rate" and ``rain rate," are set to 0.5. Other parameters align with default settings in the adopted simulation methods \cite{hahner2021fog,hahner2022lidar}.
In Universal Mixing, the preset intervals for three dimensions are set as $\Delta \rho = \frac{1}{2} (max(\rho)-min(\rho))$, $\Delta \theta= \pi$, and $\Delta z= \frac{1}{2} (max(z)-min(z))$ in spatial mixing, and $\Delta I = \frac{1}{2} (max(I)-min(I))$ in intensity mixing, where $max()$ and $min()$ denote the normalized maximum and minimum values. We chose the values of these preset interval parameters through empirical studies, which are demonstrated in the following section.

\section{Hyper-parameter Settings}\label{secB}
To investigate the effect of the hyper-parameters used in spatial mixing and intensity mixing, we conduct empirical studies regarding various hyper-parameter settings. When one hyper-parameter is varied, the remaining hyper-parameters retain their default values. As shown in Table \ref{tab:ablation_theta}, we ablate the azimuth angle interval $\Delta \theta$ with four candidate values: $1/4 \pi$, $1/2 \pi$, $ \pi$ and $3/4 \pi$. According to the experiment results, performance gains increased with the increase of the interval angle, and exchanging $180^\circ$ reaches the best mIoU improvement. We also conducted ablation studies for the radius interval $\Delta \rho$ in Table \ref{tab:ablation_rho} and $\Delta z$ in Table \ref{tab:ablation_z}, respectively. We adopt $1/4$, $1/3$, and $1/2$ intervals for both axis partitions. Experiment results indicate smaller partition ($1/4$, $1/3$) mixing is less effective than the 
 default setting  ($1/2$) in Universal Mixing. Similarly, we also conducted a parameter study for intensity mixing, as shown in Table \ref{tab:ablation_I}. Exchanging and mixing only a $1/4$ partition brings marginal improvements in both tasks. According to the empirical results, we finally set $\Delta I$ to $1/2 (max(I)-min(I))$ to obtain the largest improvement.
\section{Difference with Other Point Cloud Mixing Methods}\label{secC}
In this section, we discuss the difference between our universal mixing and other point cloud mixing methods in previous works. As shown in Table \ref{tab:comparison}, these mixing methods are proposed for mixing point clouds in different manners and addressing various tasks. CosMix \cite{saltori2022cosmix} proposes to blend point clouds by exchanging semantic patches between source data and target data, demonstrated effective in the synthetic-to-real domain adaptation task. PolarMix \cite{xiao2022polarmix} transforms point clouds to the polar coordinate and presents a data augmentation technique for point cloud representation learning by incorporating azimuth range swapping and instance-level rotate and paste. LaserMix \cite{kong2023lasermix} also divides point clouds into different partitions along inclinations in the polar coordinate and mixes two LiDAR scans in an intertwining way. Although these methods are proven effective in their tasks, none of them consider the impact of adverse weather conditions. Our universal mixing differs from these methods in the spatial partition manner and further integrates the intensity distribution-based mixing, considering the specific impacts caused by adverse weather conditions. The ablation study in Table 5 in the main paper demonstrates the superior performance of our method in both UDA and DG tasks, compared with these methods.
 
\setlength{\tabcolsep}{5.0mm}{
\begin{table}[htbp]
    \centering
    \begin{scriptsize}
    % \resizebox{0.47\textwidth}{!}{
    \begin{tabular}{c|c|c}
    \toprule
         $\Delta \theta$& \cellcolor{red!10}UDA mIoU &\cellcolor{blue!10}DG mIoU\\
    \midrule
    Source-only&24.4&24.4\\
    \midrule
    
     $1/4 \pi$ &27.2&25.1\\
    $1/2 \pi$ &31.6&25.7\\
    $3/4 \pi$ &33.2&25.9\\
    $ \pi$ &\textbf{35.2}&\textbf{26.4}\\
    \bottomrule
    \end{tabular}
    % }
    \vspace{-7pt}
    \caption{Ablation of parameter $\Delta \theta$ in spatial mixing for UDA and DG on SemanticKITTI $\rightarrow$ SemanticSTF.}
    \label{tab:ablation_theta}
    \end{scriptsize}
    \vspace{-10pt}
\end{table}
}
\setlength{\tabcolsep}{5.0mm}{
\begin{table}[htbp]
    \centering
    \begin{scriptsize}
    % \resizebox{0.47\textwidth}{!}{
    \begin{tabular}{c|c|c}
    \toprule
         $\Delta \rho$& \cellcolor{red!10}UDA mIoU &\cellcolor{blue!10}DG mIoU\\
    \midrule
    Source-only&24.4&24.4\\
    \midrule
    
     $1/4 (max(\rho)-min(\rho))$ &25.4&24.9\\
     $1/3 (max(\rho)-min(\rho))$ &28.9&25.3\\
    $1/2 (max(\rho)-min(\rho))$ &\textbf{35.2}&\textbf{26.4}\\
    
    \bottomrule
    \end{tabular}
    % }
    \vspace{-7pt}
    \caption{Ablation of parameter $\Delta \rho$ in spatial mixing for UDA and DG on SemanticKITTI $\rightarrow$ SemanticSTF.}
    \label{tab:ablation_rho}
    \end{scriptsize}
    \vspace{-10pt}
\end{table}
}
\setlength{\tabcolsep}{5.0mm}{
\begin{table}[htbp]
    \centering
    \begin{scriptsize}
    % \resizebox{0.47\textwidth}{!}{
    \begin{tabular}{c|c|c}
    \toprule
         $\Delta z$& \cellcolor{red!10}UDA mIoU &\cellcolor{blue!10}DG mIoU\\
    \midrule
    Source-only&24.4&24.4\\
    \midrule
    
     $1/4 (max(z)-min(z))$ &26.5&25.2\\
     $1/3 (max(z)-min(z))$ &29.7&25.5\\
    $1/2 (max(z)-min(z))$ &\textbf{35.2}&\textbf{26.4}\\
    
    \bottomrule
    \end{tabular}
    % }
    \vspace{-7pt}
    \caption{Ablation of parameter $\Delta z$ in spatial mixing for UDA and DG on SemanticKITTI $\rightarrow$ SemanticSTF.}
    \label{tab:ablation_z}
    \end{scriptsize}
    \vspace{-10pt}
\end{table}
}
\setlength{\tabcolsep}{5.0mm}{
\begin{table}[htbp]
    \centering
    \begin{scriptsize}
    % \resizebox{0.47\textwidth}{!}{
    \begin{tabular}{c|c|c}
    \toprule
         $\Delta I$& \cellcolor{red!10}UDA mIoU &\cellcolor{blue!10}DG mIoU\\
    \midrule
    Source-only&24.4&24.4\\
    \midrule
    
     $1/4 (max(I)-min(I))$ &26.1&24.6\\
     $1/3 (max(I)-min(I))$ &28.3&25.2\\
    $1/2 (max(I)-min(I))$ &\textbf{34.9}&\textbf{25.8}\\
    
    \bottomrule
    \end{tabular}
    % }
    \vspace{-7pt}
    \caption{Ablation of parameter $\Delta I$ in spatial mixing for UDA and DG on SemanticKITTI $\rightarrow$ SemanticSTF.}
    \label{tab:ablation_I}
    \end{scriptsize}
    \vspace{-10pt}
\end{table}
}

\setlength{\tabcolsep}{0.2mm}{
\begin{table}[htbp]
    \centering
    \begin{scriptsize}
    \resizebox{0.47\textwidth}{!}{
    \begin{tabular}{c|c|c|c|c}
    \toprule
         method&spatial (coordinate, partition) &semantic&intensity&task\\
    \midrule

    CosMix \cite{saltori2022cosmix} &&$\checkmark$ &&Syn-to-real UDA\\
    PolarMix \cite{xiao2022polarmix} &$\checkmark$ (Polar,inclination)  &$\checkmark$  &&Data augmentation\\
    LaserMix \cite{kong2023lasermix} &$\checkmark$ (Polar, azimuth) &  &&Semi-supervised LSS\\
    Universal Mixing &$\checkmark$ (Cylinder (radius, azimuth, z)) &$\checkmark$  &$\checkmark$&clear-to-adverse UDA and DG\\
    
    \bottomrule
    \end{tabular}
    }
    \vspace{-7pt}
    \caption{Comparison of various mixing methods.}
    \label{tab:comparison}
    \end{scriptsize}
    \vspace{-10pt}
\end{table}
}

\section{Bridge Domain Visualization}\label{secD}
During Bridge Domain construction, we simulate frequent four weather conditions for each scene. However, we load Bridge domain data by randomly selecting a single weather condition in the training phases.

In Fig. \ref{figure:simueffect_supp}, we show the simulated examples in the Bridge Domain in diverse weather conditions. All adverse weather conditions introduce disturbance particles but in different patterns. Light fog and dense fog cause surround noisy points with different densities while rain and snow bring irregular scattering particles.

\begin{figure}[htbp]
    \begin{center}
    \includegraphics[width=\linewidth]{figures/weather simulation.pdf}
    \end{center}
    \vspace{-0.5cm}
    \caption{Visualization of the simulated bridge domain in four weather conditions.}
    \label{figure:simueffect_supp}
    \vspace{-0.3cm}
\end{figure}

\section{Intermediate Point Cloud Visualization}\label{secE}
In Fig. \ref{figure:mixingVis_supp}, we show the mixed intermediate point clouds using different mixing methods, including semantic mixing, spatial mixing, and intensity mixing. To illustrate the point clouds clearly, we show the spatial mixing regarding three dimensions. As shown in Fig. \ref{figure:mixingVis_supp}, the mixing methods can effectively create intermediate point clouds with high diversity, facilitating learning weather-robust representations.
\begin{figure*}[t]
    \begin{center}
    \includegraphics[width=0.83\linewidth]{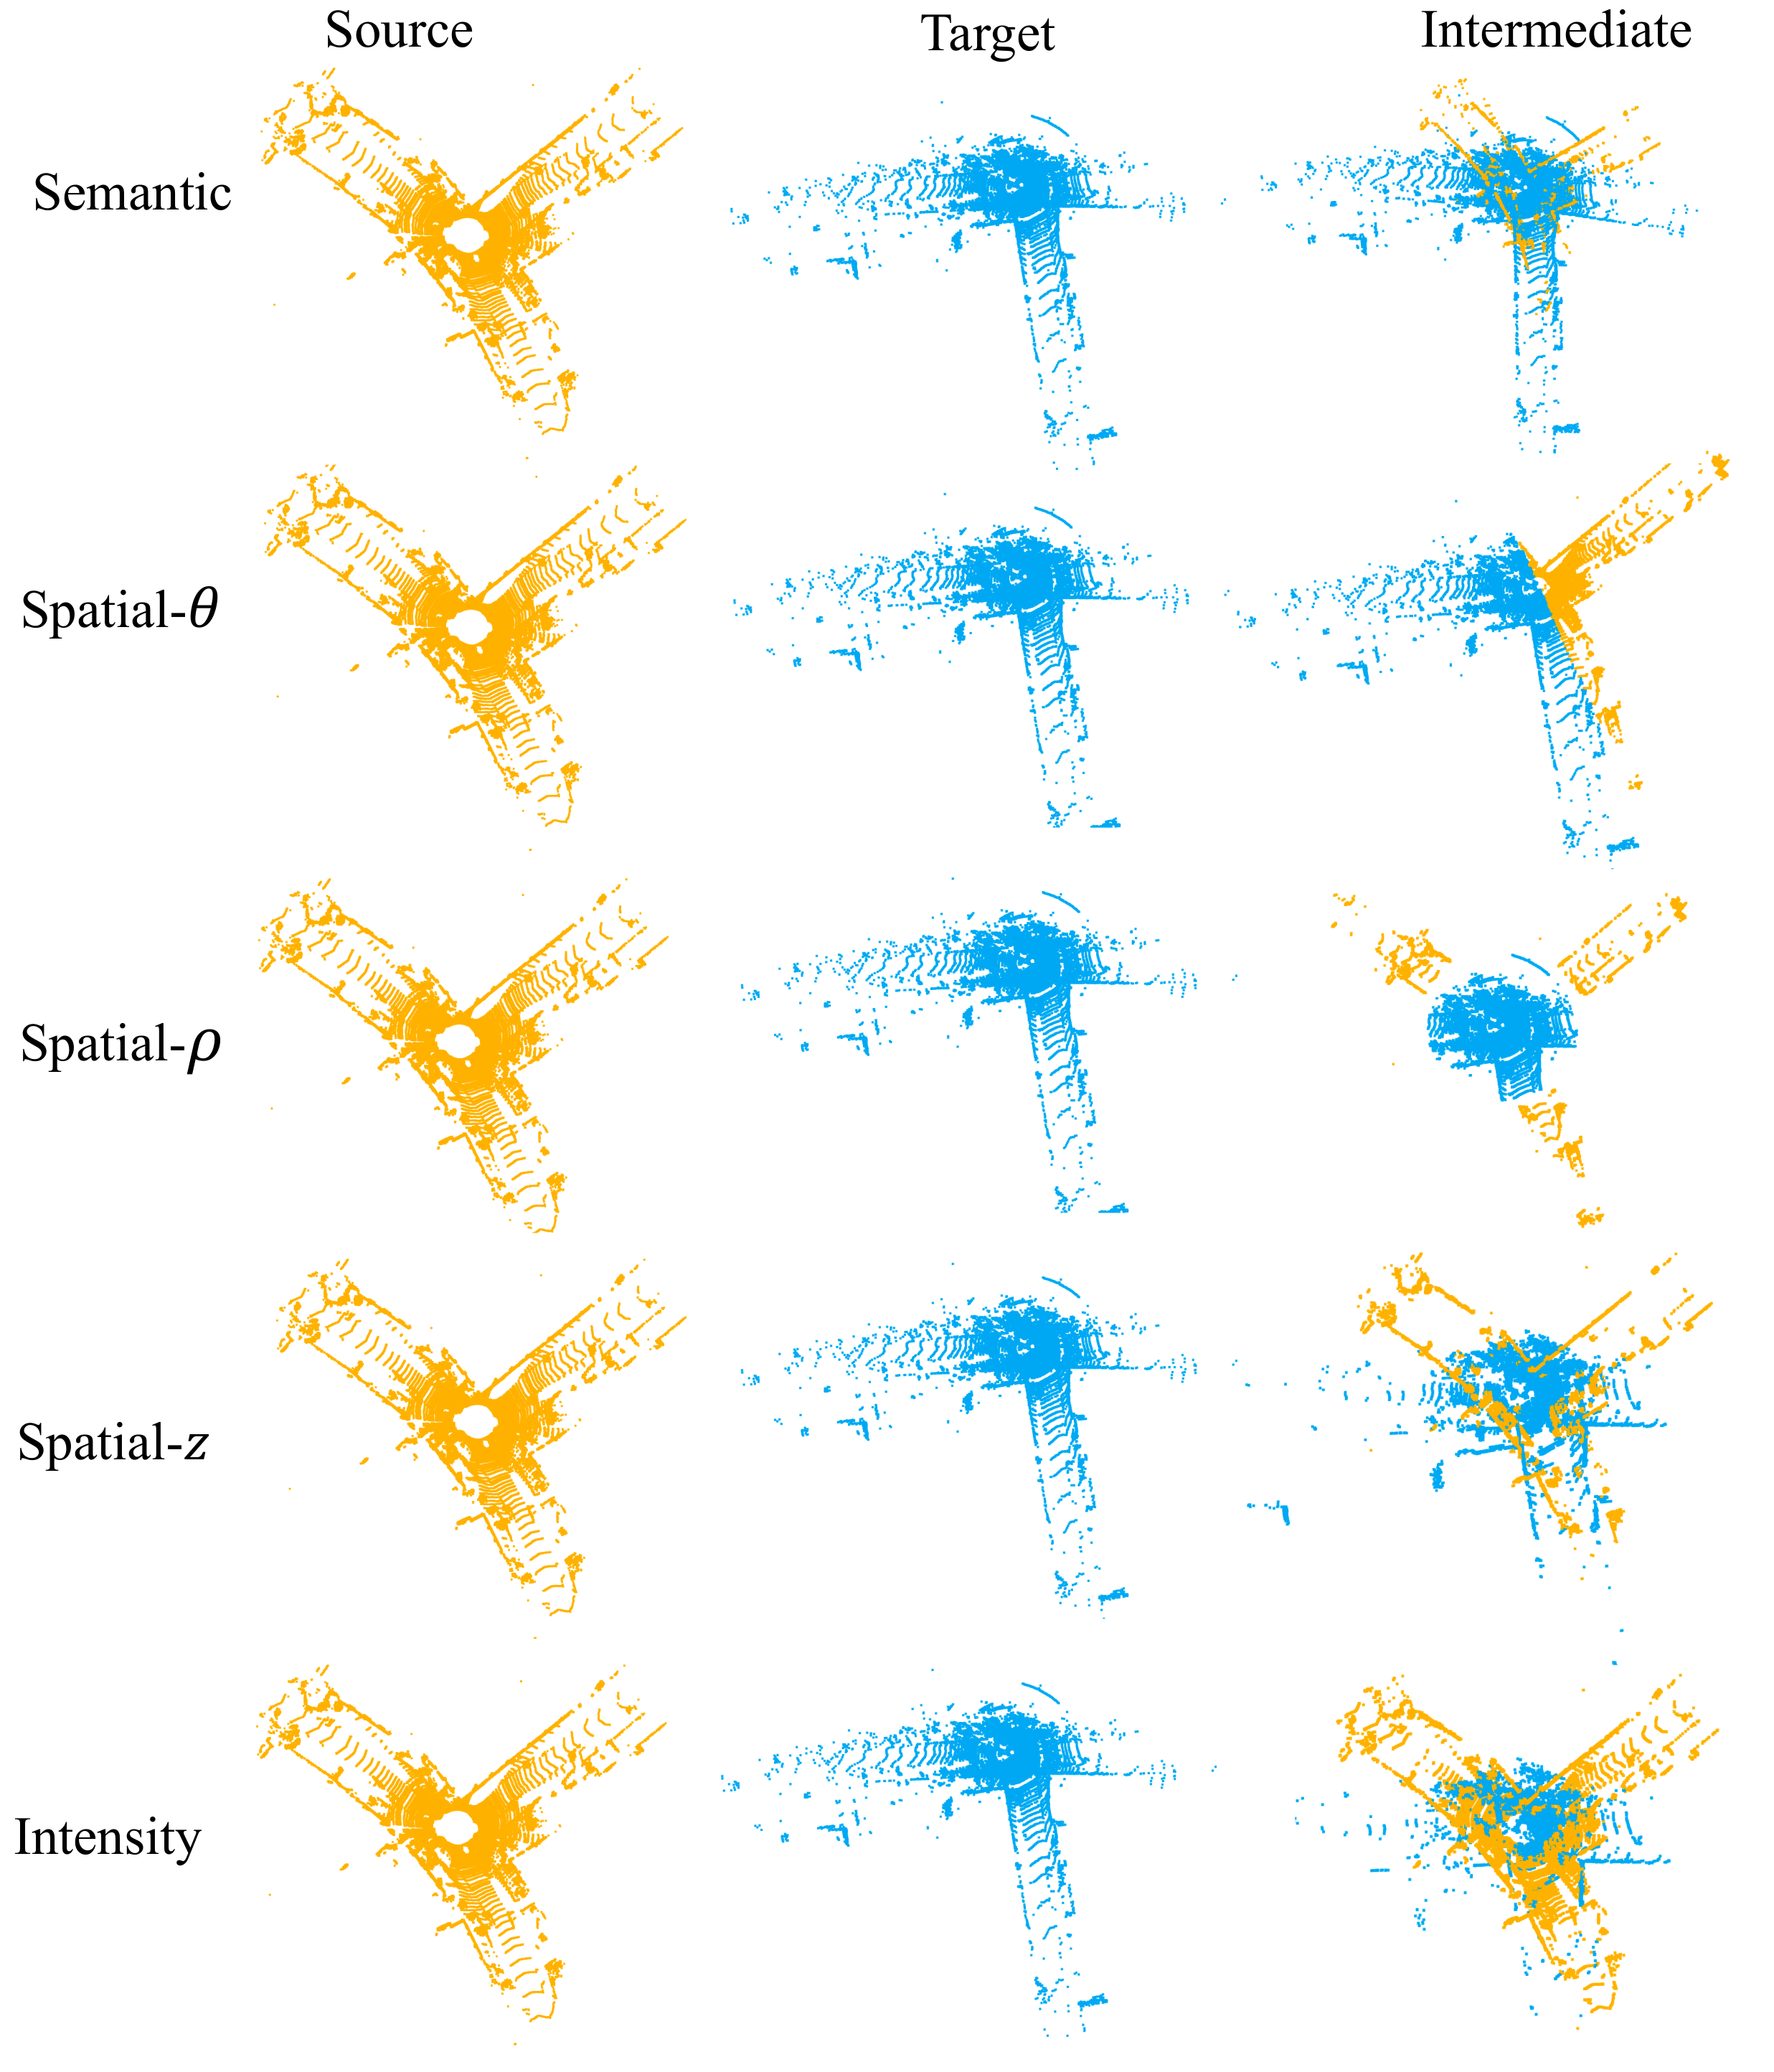}
    \end{center}
    \vspace{-0.5cm}
    \caption{Visualization of the mixed intermediate point clouds. The point clouds in yellow and blue are samples from source and target data, respectively. We show the mixed intermediate point clouds generated by different mixing methods.}
    \label{figure:mixingVis_supp} 
    \vspace{-0.3cm}
\end{figure*}

\section{Qualitative Results}\label{secF}
\label{sec:rationale}
In Fig. \ref{figure:QualiVis_supp}, we show some qualitative LiDAR segmentation results of our method, including the ground truth, results after UDA, results after DG, and the results of the source-only model, respectively. Due to the severe disturbance of adverse weather conditions, the LiDAR scans are generally different from those in clear weather, leading to numerous floating points (row 2) and LiDAR scan incompleteness (rows 3 and 4). As shown in Fig. \ref{figure:QualiVis_supp}, we highlight the significant distinctions between different results with blue circles. The color map is displayed at the bottom. The UDA model produces better qualitative results than the DG model, which both largely outperform the source-only model. However, the segmentation results are not that satisfactory, indicating a large room for improvement in the adverse-weather benchmarks. We hope our method can provide valuable insights into future research on perception and understanding in adverse weather.

\begin{figure*}[t]
    \begin{center}
    \includegraphics[width=0.95\linewidth]{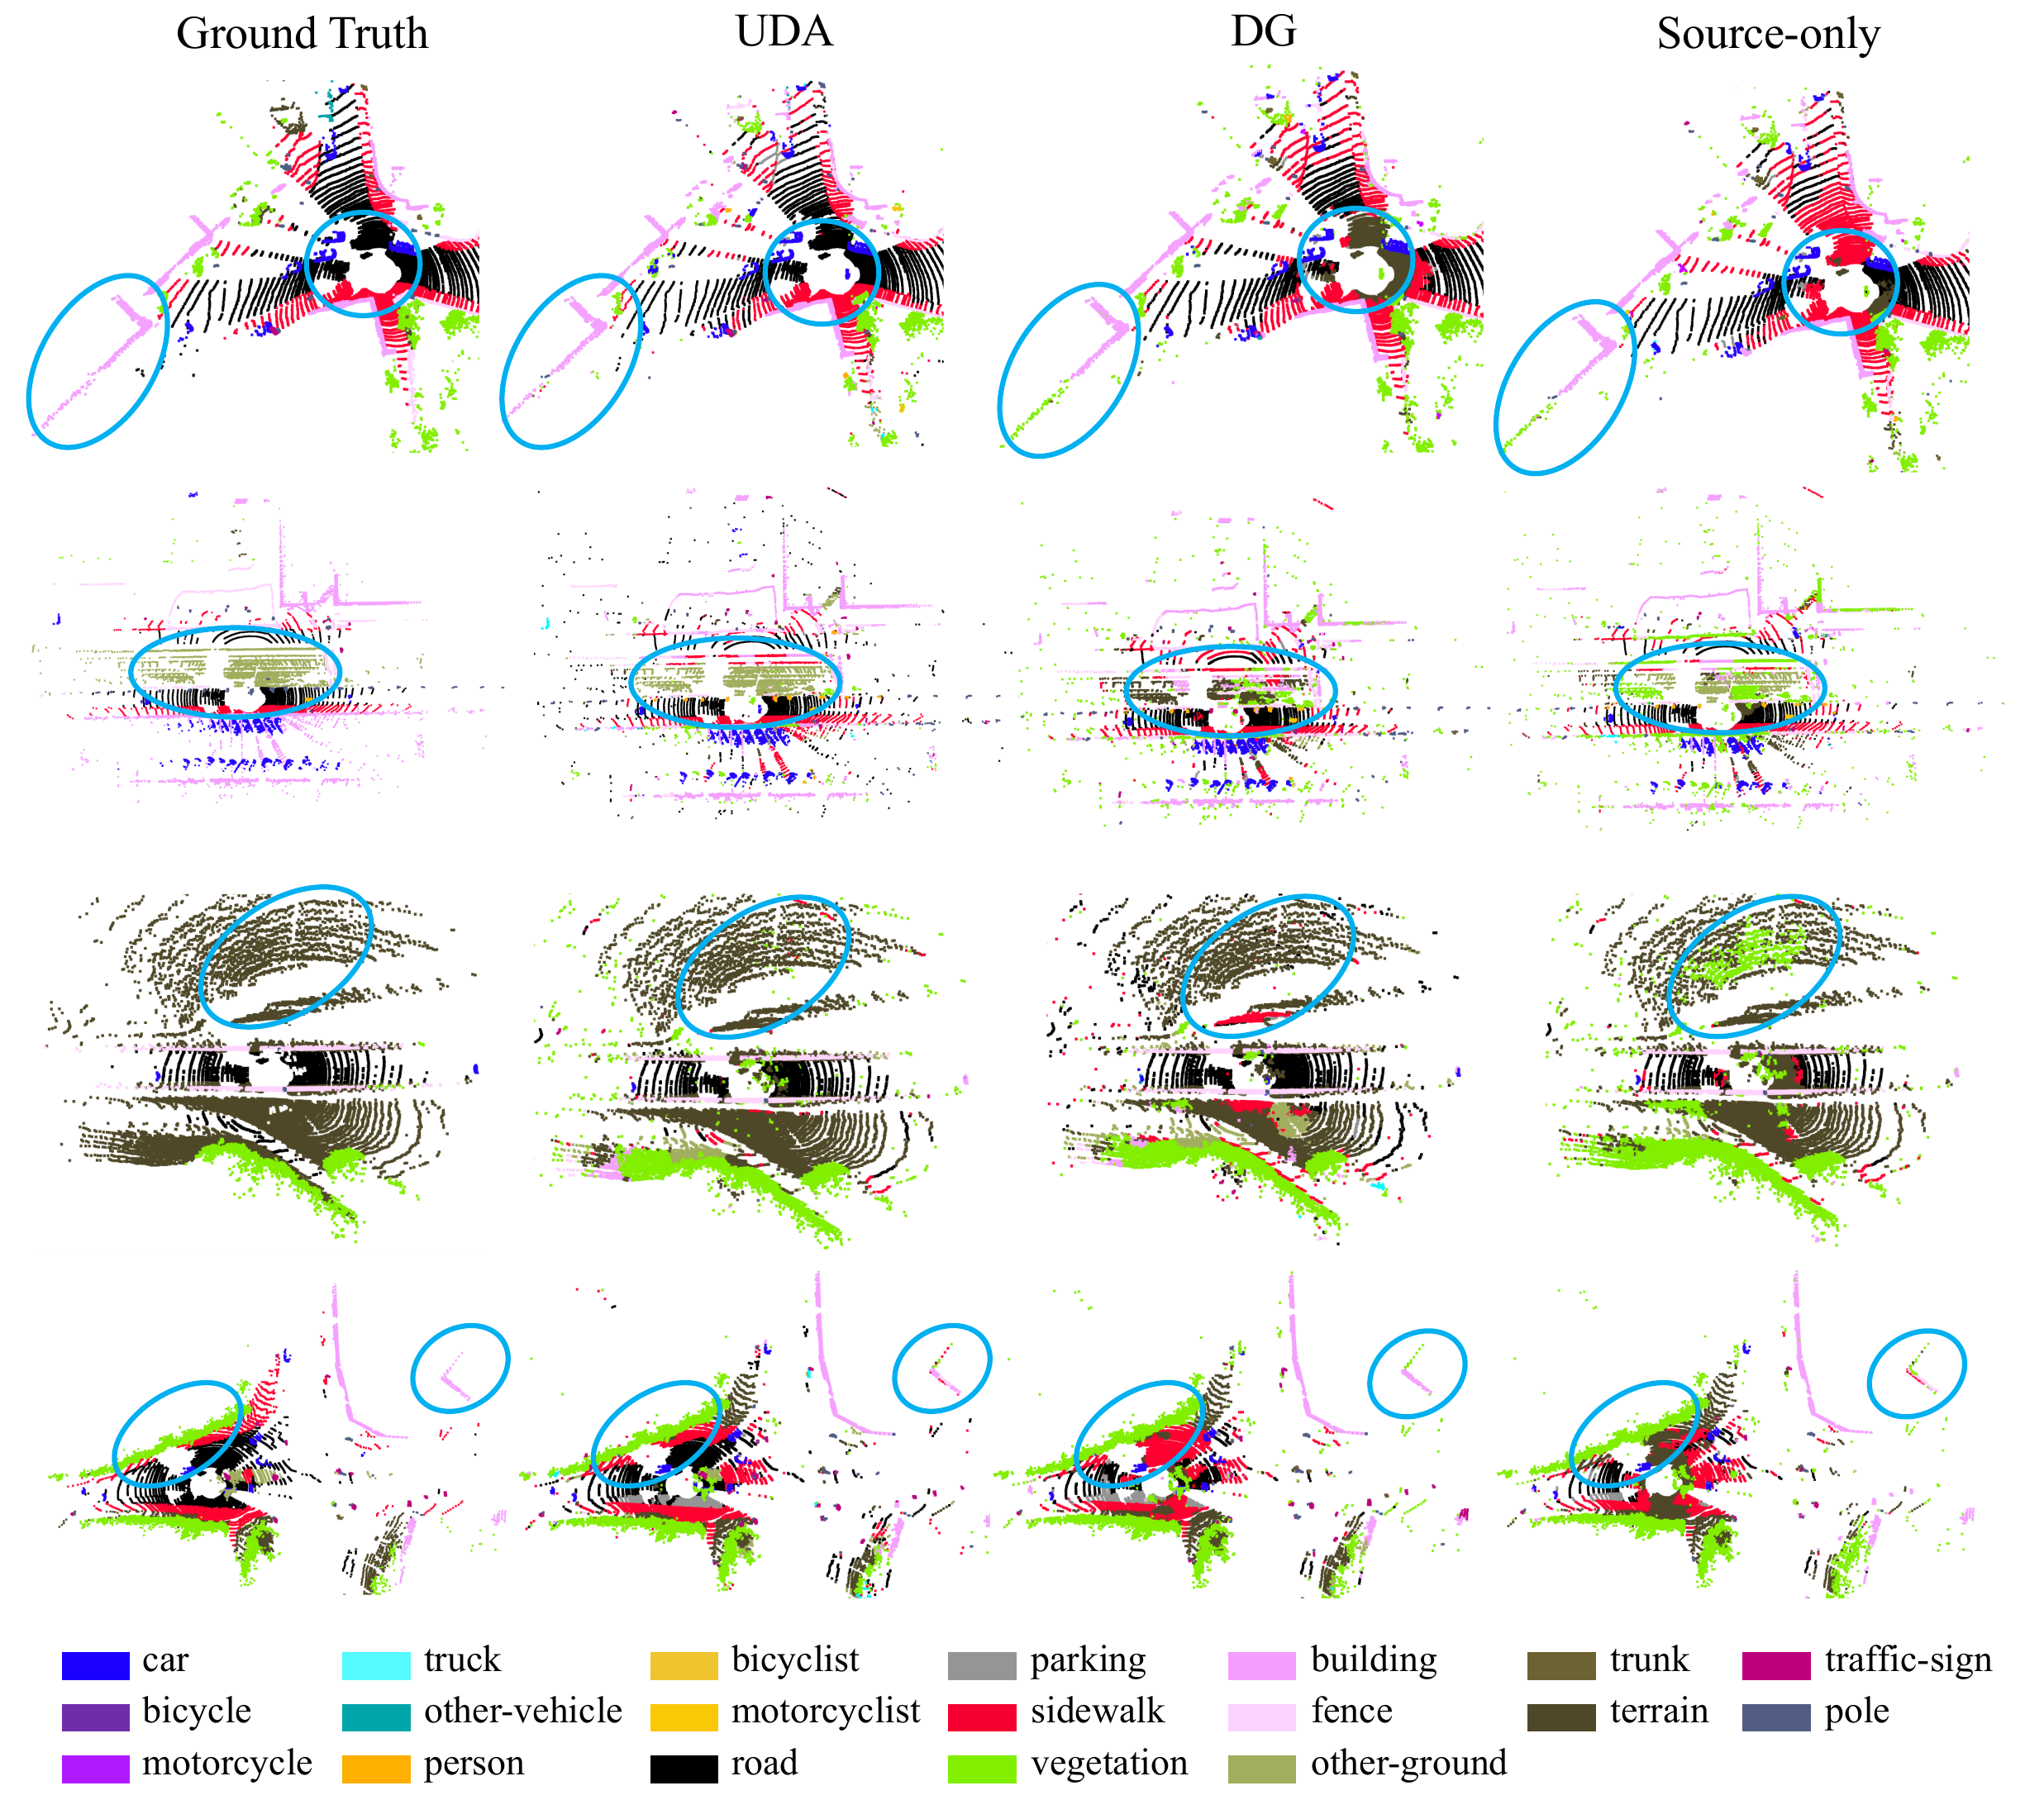}
    \end{center}
    \vspace{-0.5cm}
    \caption{Qualitative results on SemanticKITTI$\rightarrow$SemanticSTF. We display the ground truth, results after domain adaptation and domain generalization, and results of the source-only model. We highlight the significant distinctions between different results with blue circles. The color map is displayed at the bottom. Best viewed with zoom-in and in color.}
    \label{figure:QualiVis_supp}
    \vspace{-0.3cm}
\end{figure*}
% \section{Feature Visualization}\label{secG}

\section{Limitations and Social Impact}\label{secH}
While UniMix shows effective in enhancing the adaptability and generalizability of LiDAR semantic segmentation (LSS) models, it is essential to acknowledge potential limitations and consider their broader societal implications. First, there is still a large room for improvement in the adverse-weather LiDAR semantic segmentation benchmarks. Since some self-supervised pre-training techniques \cite{pang2022masked,Tian_2023_CVPR} have been demonstrated effective in several related tasks such as part segmentation and 3D object detection, it is worth trying to employ these pre-training approaches to obtain generalizable feature representation as a good starting point to further improve performance.
%We hope our method could provide valuable insights for future adverse-weather 3D perception and understanding works. 
%Second, the method's effectiveness may be contingent on the realism of the adverse weather simulation and the representativeness of the constructed Bridge Domain. Inaccuracies in simulating certain weather conditions or potential biases in the training data could impact the model's performance in real-world scenarios. 
Besides, like many UDA methods, the two-stage training of UniMix brings a little more computational cost, although it provides a complete and competitive solution for both DG and UDA tasks. 

LiDAR is presently the most commonly used and effective sensor in autonomous driving systems and LiDAR semantic segmentation constitutes the foundational task in scene perception. However, adverse weather conditions severely interfere with LiDAR, rendering existing models ineffective. While our method has demonstrated the ability to enhance the model's capacity to learn weather-robust and domain-invariant representations, improving the system's resilience to adverse weather conditions remains an open challenge that is worth exploring for ensuring safety and reliability in real applications.
%Regarding social impact, privacy and algorithm security concerns, especially in deploying LSS models in autonomous driving, warrant attention. Ensuring fair, unbiased behavior in diverse contexts requires prioritizing ethical considerations. As UniMix and similar technologies evolve, a proactive, inclusive approach is vital for responsible and equitable deployment in autonomous systems.

% 
% Having the supplementary compiled together with the main paper means that:
% % 
% \begin{itemize}
% \item The supplementary can back-reference sections of the main paper, for example, we can refer to \cref{sec:intro};
% \item The main paper can forward reference sub-sections within the supplementary explicitly (e.g. referring to a particular experiment); 
% \item When submitted to arXiv, the supplementary will already included at the end of the paper.
% \end{itemize}
% % 
% To split the supplementary pages from the main paper, you can use \href{https://support.apple.com/en-ca/guide/preview/prvw11793/mac#:~:text=Delete%20a%20page%20from%20a,or%20choose%20Edit%20%3E%20Delete).}{Preview (on macOS)}, \href{https://www.adobe.com/acrobat/how-to/delete-pages-from-pdf.html#:~:text=Choose%20%E2%80%9CTools%E2%80%9D%20%3E%20%E2%80%9COrganize,or%20pages%20from%20the%20file.}{Adobe Acrobat} (on all OSs), as well as \href{https://superuser.com/questions/517986/is-it-possible-to-delete-some-pages-of-a-pdf-document}{command line tools}.
